# Supplementary material for: Sequence to Sequence Mixture Model for Diverse Machine Translation
Source: arXiv:1810.07391 source file (2018-10-17)
Supplement: Supplementary file 1 [file supp.tex]

%
% File emnlp2018.tex
%
%% Based on the style files for EMNLP 2018, which were
%% Based on the style files for ACL 2018, which were
%% Based on the style files for ACL-2015, with some improvements
%%  taken from the NAACL-2016 style
%% Based on the style files for ACL-2014, which were, in turn,
%% based on ACL-2013, ACL-2012, ACL-2011, ACL-2010, ACL-IJCNLP-2009,
%% EACL-2009, IJCNLP-2008...
%% Based on the style files for EACL 2006 by 
%%e.agirre@ehu.es or Sergi.Balari@uab.es
%% and that of ACL 08 by Joakim Nivre and Noah Smith

\documentclass[11pt,a4paper]{article}
\usepackage[hyperref]{conll2018}
\usepackage{times}
\usepackage{latexsym}
\usepackage{amssymb}
\usepackage[fleqn]{amsmath}
\usepackage{graphicx}
\usepackage{algorithm}  
\usepackage{algorithmic}
\usepackage{multirow}
\usepackage{array}
\usepackage{pifont}
\graphicspath{{figures/}}
\usepackage{subcaption}
\usepackage[utf8]{vietnam}

\usepackage{url}
\input{defs}

\aclfinalcopy % Uncomment this line for the final submission
%\def\aclpaperid{***} %  Enter the acl Paper ID here

%\setlength\titlebox{5cm}
% You can expand the titlebox if you need extra space
% to show all the authors. Please do not make the titlebox
% smaller than 5cm (the original size); we will check this
% in the camera-ready version and ask you to change it back.

\title{Supplementary Material  \\ Sequence to Sequence Mixture Model~~for~~Diverse Machine Translation
% Neural Machine Translation of Heterogeneous Text \\ with Mixture of Sequence to Sequence Models
}

\date{}

\begin{document}
\maketitle

\section{ $n$-gram Diversity Measures}
\input{supp-div.tex}

\section{Distribution Among Mixture Copmonents}
\input{supp-dist.tex}

\section{Qualitative Examples}
\input{supp-qual.tex}
\end{document}
